# Supplementary material for: Parameterized Saga of First-Fit and Last-Fit Coloring
Source: arXiv:2410.20629 source file (2024-10-27)
Supplement: Supplementary file 1 [file additional-proofs.tex]

\begin{observation}\label{obs:grundy-witness-closure}
Consider $k \in \mathbb{N}\setminus \{0\}$, a graph $G$ and a $k$-Grundy witness ${\sf wit}: V(T_k) \rightarrow V(G)$ for $G$. For each $q \in [k-1]$, ${\sf wit}|_{V(T_{q})}$ is a $q$-Grundy witness for $G$. 
\end{observation}
\begin{proof}
Let  ${\sf wit}: V(T_k) \rightarrow V(G)$ be a   $k$-Grundy witness for $G$. Then by Definition \ref{def:grundy-witness-uncol}, for each $q\in [k]$,  $\{{\sf wit}(t) \mid t \in V(T_k) \mbox{ and } \ell_k(t) = q\}$ is an independent set in $G$. It implies that for any $q\in[k-1]$ and $r\in [q]$,  $\{{\sf wit}(t) \mid t \in V(T_q) \mbox{ and } \ell_q(t) = r\}$ is an independent set in $G$ as $\ell_k(t)=\ell_r(t)$ by Definition \ref{def:grundy-tree-new}. Since $T_q$ is a subtree of tree $T_k$ for any $q\in [k-1]$, properties $2$ and $3$ of Definition \ref{def:grundy-witness-uncol} holds for each $t,t'\in V(T_q)$ and $(t,t')\in E(T_q)$. Hence, ${\sf wit}|_{V(T_{q})}$ is a $q$-Grundy witness for $G$ for each $q\in [k-1]$.
\end{proof}

\begin{observation}\label{obs:good-prob}
The coloring $\chi$ is nice with probability at least {\em blah}.
\end{observation}
\begin{proof}
The coloring $\chi$ is nice, if for each $q\in [k]$ and $v\in \what{V}_{{\sf wit},q}$, $\chi(v)=q$. Note that the size of $\what{V}_{{\sf wit},q}$ is same as the number of subtrees $T_q$ in $T_k$, that is, $2^{k-(q+1)}$, for any $q\in[k-1]$. Moreover, the size of $\what{V}_{{\sf wit},k}$ is $1$. Now, the probability that the coloring $\chi$ assigns the color $q$ to all the vertices in $\what{V}_{{\sf wit},q}$ ia at least $\frac{1}{k}^{|\what{V}_{{\sf wit},q}|}$.  Therefore, the probability that the coloring $\chi$ is nice,
\begin{equation*}

 & = \Pi_{q=1}^{k} \mbox {Pr[vertices of } \what{V}_{{\sf wit},q} \mbox{ are colored with color } q]\\
& \geq  \Pi_{q=1}^{k}  \frac{1}{k}^{|\what{V}_{{\sf wit},q}|}\\
& \geq  \Pi_{q=1}^{k-1}  (\frac{1}{k})^{2^{k-(q+1)}}\cdot \frac{1}{k} \geq (\frac{1}{k})^{2^{k^2}}.

\end{equation*}
\end{proof}

\begin{observation}\label{obs:transitive-vec-rep}
Consider $p \in \mathbb{N}$, a vector $\vec{q} = (q_1,q_2,\cdots, q_k)$, and (not necessarily disjoint) $p$-families $\C{F}_1$ and $\C{F}_2$. If $\C{F}'_1 \subseteq^{\vec{q}}_{grep} \C{F}_1$ and $\C{F}'_2 \subseteq^{\vec{q}}_{grep} \C{F}_2$, then $\C{F}'_1 \cup \C{F}'_2 \subseteq^{\vec{q}}_{grep} \C{F}_1 \cup \C{F}_2$. 
\end{observation}

\begin{proof}
Consider a set $B$ of size $\vec{q}$ such that there is some set $A\in \C{F}_1\cup \C{F}_2$ that fits $B$. If $A\in \C{F}_1$, then there exists some $A'\in \C{F}'_1$ that fits $B$ as $\C{F}'_1 \subseteq^{\vec{q}}_{grep} \C{F}_1$. If $A\in \C{F}_2$, then there exists some $A'\in \C{F}'_2$ that fits $B$ as $\C{F}'_2 \subseteq^{\vec{q}}_{grep} \C{F}_2$. Thus, there exists $A'\in \C{F}'_1\cup\C{F}'_2$ that fits $B$. Hence, $\C{F}'_1 \cup \C{F}'_2 \subseteq^{\vec{q}}_{grep} \C{F}_1 \cup \C{F}_2$.
\end{proof}

\begin{observation}\label{obs:transitive-vec-rep-one-vertex}
Consider $p \in \mathbb{N}$, a vector $\wvec{q} = (q_1,q_2,\cdots, q_k)$, a vertex $v \in V(G)$ and a $(p,v)$-family $\C{F}$. Let $\wvec{h}$ be the vector obtained from $\wvec{q}$ by increasing its $\chi(v)$th coordinate by $1$. If $\C{F}' \qrep{h} \C{F}-v$, then $\C{F}' + v \qrep{q} \C{F}$. 
\end{observation}

\begin{proof}
Consider a set $B$ of size $\vec{q}$ such that there is some set $A\in \C{F}$ that fits $B$. Since $\C{F}$ is a $(p,v)$-family, $v\in A$. Clearly, $A\setminus \{v\}\in \C{F}-v$ and $B\setminus \{v\}$ is of size $\vec{h}$. Now, there exists a set $A'\in \C{F}'$ that fits $B\setminus \{v\}$ as $\C{F}'\qrep{h} \C{F}-v$. It follows that $A'\cup\{v\} \in \C{F}'+v $ and $A'\cup\{v\} $ fits $B$. Hence, $\C{F}' + v \qrep{q} \C{F}$.
\end{proof}
